# Supplementary material for: Chain-of-Layer: Iteratively Prompting Large Language Models for Taxonomy Induction from Limited Examples
Source: arXiv:2402.07386 source file (2024-07-25)
Supplement: Supplementary file 1 [file 7appendix_case_study.tex]

\section{Case Study}
\label{app:case}
In this section, we present a case study that illustrates the strengths and weaknesses between our proposed methods and several baselines. We select samples from WordNet and present the outputs of \textsc{CoL}, \textsc{CoL-Zero}, \textsc{CoL-w/o-Filter}, \textsc{HF (GPT-4)} and \textsc{HF (GPT-4)-Filter} in the 5-shot setting.

\subsection{\textsc{CoL} / \textsc{CoL-Zero} v.s. Ground Truth}
Comparing the taxonomies induced by the \textsc{CoL} (Figure \ref{fig:case_1} b) and \textsc{CoL-Zero} (Figure \ref{fig:case_1} c) against the ground truth (Figure \ref{fig:case_1} a), we can observe several differences and potential reasons behind these discrepancies.

\paragraph{Differences between CoL and CoL-Zero:} In the provided case, the taxonomy induced by \textsc{CoL} follows a more traditional organization closely related to the ground truth, with cutlery divided into spoons, forks, and knives, each having further specialization. \textsc{CoL-Zero} seems to treat each item more independently and does not adhere strictly to the conventional grouping of cutlery (e.g., ``separating fish knife'', ``butter knife'', ``steak knife'', etc., into distinct categories without grouping them under a single ``table knife'' category).

\paragraph{Differences from the Ground Truth:} Compared to ground truth, \textsc{CoL} achieves 0.9048 in edge F1-score and \textsc{CoL-Zero} achieves 0.6667. A common type of error caused by LLMs' incorrect understanding of certain concepts, or the ambiguity inherent in the concepts themselves. For example, both \textsc{CoL} and \textsc{CoL-Zero} suggest that ``tea maker'' is not a type of spoon but a direct type of cutlery. In this case, ``tea maker'' refers to ``a perforated covered spoon that holds tea leaves and is used in brewing tea in a cup.'', instead of another type of cutlery that can be used to make tea.

Another type of error involves issues with the granularity of grouping, specifically whether two concepts should be classified in a hierarchical relationship or as siblings. Taking the taxonomy induced by \textsc{CoL} as an example, ``iced-tea spoon'' is classified as a type of spoon, instead of a type of ``teaspoon''. Such errors could occur when generating the $k_{th}$ layer, which only considers the relationship between the entities in $\mathcal{V}_{sel}$ and those in the ${(k-1)}_{th}$ layer, without take the relationships among the entities within $\mathcal{V}_{sel}$ itself into careful consideration.
% Ground Truth:
% 1. cutlery
% 1.1 Spork
% 1.2 table knife
% 1.2.1 case knife
% 1.2.2 steak knife
% 1.2.3 butter knife
% 1.2.4 fish knife
% 1.3 spoon
% 1.3.1 teaspoon
% 1.3.1.1 iced-tea spoon
% 1.3.2 soupspoon
% 1.3.3 sugar spoon
% 1.3.4 dessert spoon
% 1.3.5 runcible spoon
% 1.3.6 tea maker
% 1.3.7 wooden spoon
% 1.3.8 tablespoon
% 1.4 fork
% 1.4.1 salad fork
% 1.4.2 tablefork
% 1.4.3 carving fork
% 1.4.4 toasting fork

% CoL: 
% 1. cutlery
% 1.1 spork
% 1.2 table knife
% 1.2.1 steak knife
% 1.2.2 fish knife
% 1.2.3 butter knife
% 1.2.4 case knife
% 1.3 spoon
% 1.3.1 iced-tea spoon
% 1.3.2 soupspoon
% 1.3.3 teaspoon
% 1.3.4 dessert spoon
% 1.3.5 runcible spoon
% 1.3.6 wooden spoon
% 1.3.7 sugar spoon
% 1.3.8 tablespoon
% 1.4 tea maker
% 1.5 fork
% 1.5.1 tablefork
% 1.5.2 salad fork
% 1.5.3 toasting fork
% 1.5.4 carving fork

% CoL-Zero:
% 1. cutlery
% 1.1 spoon
% 1.1.1 soupspoon
% 1.1.2 iced-tea spoon
% 1.1.3 runcible spoon
% 1.1.4 dessert spoon
% 1.1.5 tablespoon
% 1.1.6 wooden spoon
% 1.1.7 sugar spoon
% 1.1.8 teaspoon
% 1.2 toasting fork
% 1.3 fish knife
% 1.4 tea maker
% 1.5 butter knife
% 1.6 table knife
% 1.7 case knife
% 1.8 spork
% 1.9 fork
% 1.9.1 tablefork
% 1.9.2 carving fork
% 1.9.3 salad fork
% 1.10 steak knife

\subsection{CoL v.s. CoL-w/o-Filter}
To better illustrate the role of the ensemble-based ranking rilter, we compare the outputs of \textsc{CoL} (Figure \ref{fig:case_2} b) and \textsc{CoL-w/o-Filter} (Figure \ref{fig:case_2} c), analyzing their differences with the ground truth (Figure \ref{fig:case_2} a). As shown in Figure \ref{fig:case_2}, the taxonomy induced by \textsc{CoL} is very close to ground truth, while \textsc{CoL-w/o-Filter} mis-classify ``roll'', ``bank'', and ``loop'' as siblings of ``flight maneuvers''. This to some extent proves the effectiveness of our ensemble-based ranking rilter, which functions to filter out edges with lower filter ranks, such as ``flight maneuvers - roll'', and then re-adds ``roll'' to $\mathcal{V}_k$ for selection when generating the next layer. Such a self-correcting process can help the LLM induce a more reasonable taxonomy.

% Ground Truth:
% 1. maneuver
% 1.1 straight-arm
% 1.2 flight maneuver
% 1.2.1 roll
% 1.2.1.1 snap roll
% 1.2.1.2 barrel roll
% 1.2.2 loop
% 1.2.2.1 outside loop
% 1.2.2.2 inside loop
% 1.2.3 bank
% 1.2.3.1 vertical bank
% 1.2.4 chandelle
% 1.2.5 slip
% 1.3 clinch

% CoL:
% 1. maneuver
% 1.1 straight-arm
% 1.2 flight maneuver
% 1.2.1 loop
% 1.2.1.1 inside loop
% 1.2.1.2 outside loop
% 1.2.2 slip
% 1.2.3 bank
% 1.2.3.1 chandelle
% 1.2.3.2 vertical bank
% 1.2.4 roll
% 1.2.4.1 barrel roll
% 1.2.4.2 snap roll
% 1.3 clinch

% CoL-No-Filter
% 1. maneuver
% 1.1 clinch
% 1.1.1 straight-arm
% 1.2 bank
% 1.2.1 vertical bank
% 1.3 loop
% 1.3.1 outside loop
% 1.3.2 inside loop
% 1.4 roll
% 1.4.1 barrel roll
% 1.4.2 snap roll
% 1.5 flight maneuver
% 1.5.1 chandelle
% 1.5.2 slip

\subsection{CoL v.s. HF (GPT-4) / HF-Filter (GPT-4)}
In this part, by comparing the outputs of the \textsc{CoL} (Figure \ref{fig:case_3} a)  and \textsc{HF (GPT-4)} (Figure \ref{fig:case_2} b) / \textsc{HF (GPT-4)-Filter} (Figure \ref{fig:case_2} c), we demonstrate the effectiveness and importance of our \textsc{CoL} approach and the ensemble-based ranking rilter. Compared to the ground truth, the most noticeable issue with \textsc{HF (GPT-4)}'s output is that it hallucinates an entity `knife' that wasn't in the entity list and uses it to group all other entities that should belong to `table knife'. This resulted in a lower edge F1 score for the generated taxonomy. 

By comparing the outputs of \textsc{HF (GPT-4)} and \textsc{HF (GPT-4)-Filter}, we can demonstrate that, if we do not have a layer-by-layer decomposition approach like the \textsc{CoL}, directly employing a filter would likely impair the quality of the induced taxonomy. We can observe that after directly filtering \textsc{HF (GPT-4)}'s output, the entire sub-taxonomy under `knife' was filtered out. This type of issue causes significant damage to the node F1 score of the generated taxonomy because these filtered entities cannot be re-selected, leading to a decrease in the edge F1 score.  These examples once again demonstrate the importance and synergistic effect of the \textsc{CoL} and the Ensemble-based Ranking Filter.

% Direct:
% 1. cutlery
% 1.1 spoon
% 1.1.1 soupspoon
% 1.1.2 wooden spoon
% 1.1.3 teaspoon
% 1.1.4 sugar spoon
% 1.1.5 runcible spoon
% 1.1.6 iced-tea spoon
% 1.1.7 dessert spoon
% 1.1.8 tablespoon
% 1.1.9 Spork
% 1.2 fork
% 1.2.1 tablefork
% 1.2.2 salad fork
% 1.2.3 carving fork
% 1.2.4 toasting fork
% 1.3 knife
% 1.3.1 table knife
% 1.3.2 butter knife
% 1.3.3 fish knife
% 1.3.4 steak knife
% 1.3.5 case knife
% 1.4 tea maker

% \begin{figure*}[htbp]
%     \centering
%         \includegraphics[width=1\textwidth]{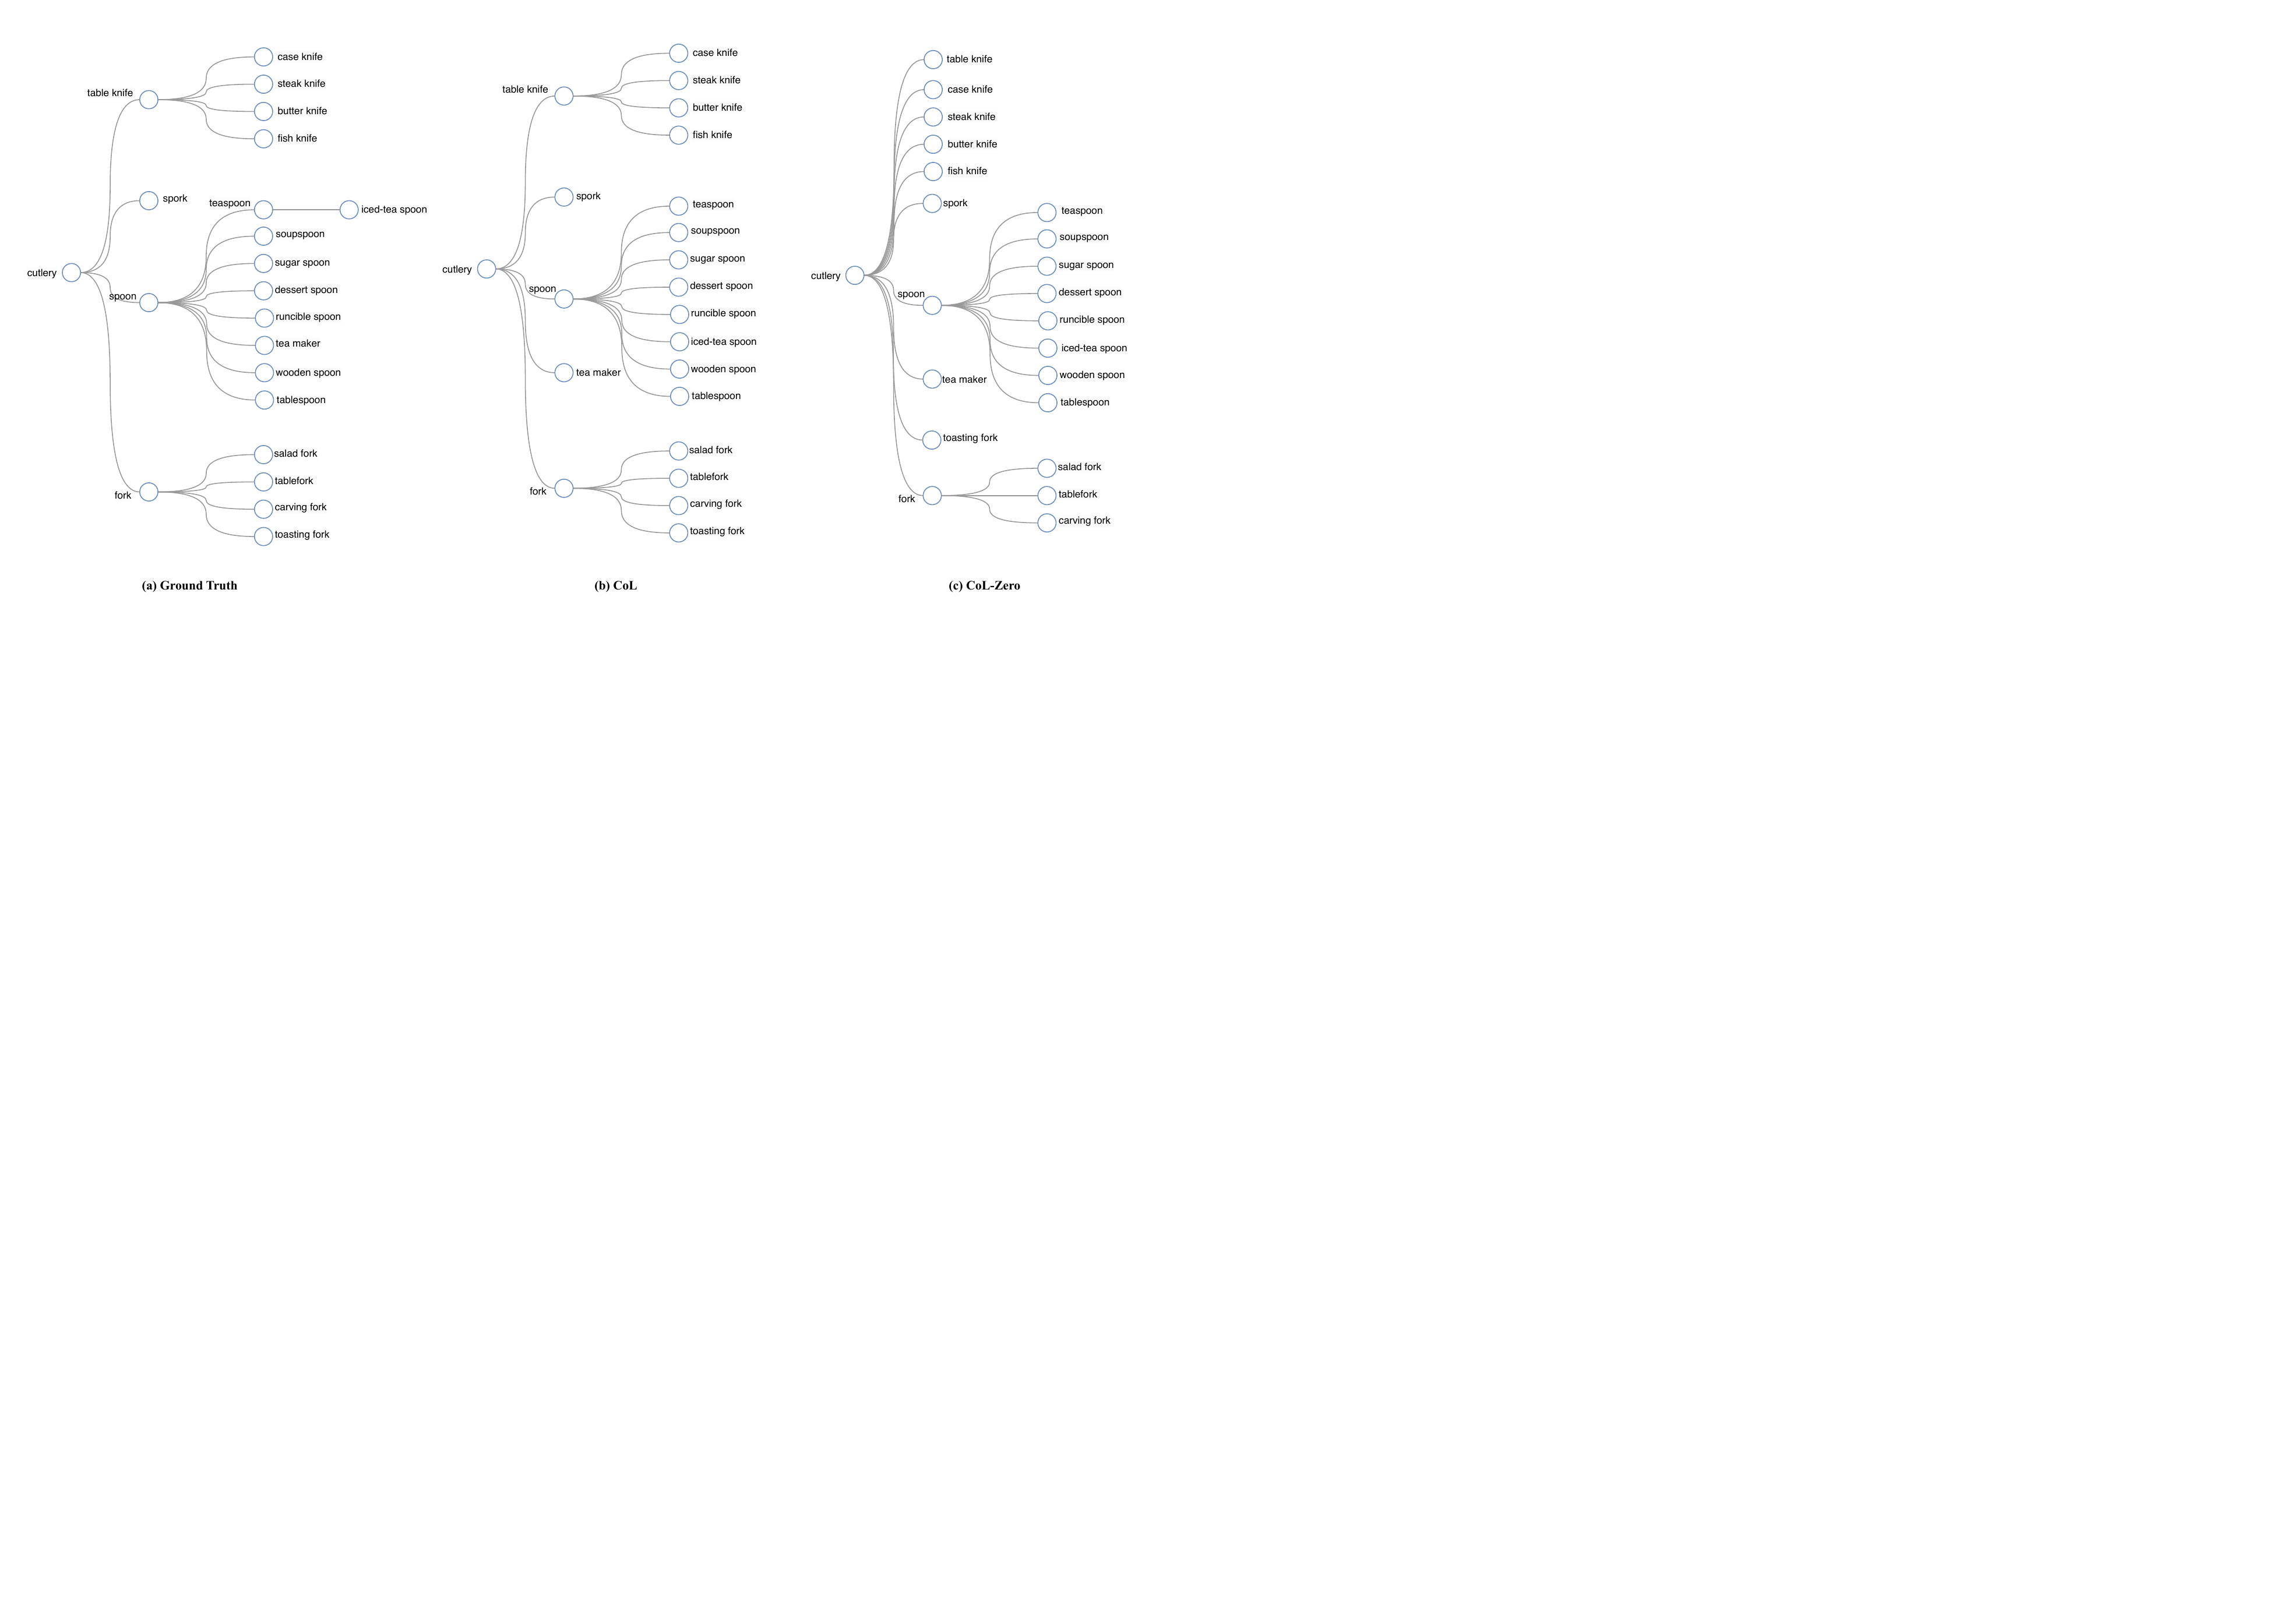}
%     \caption{CoL / CoL-Zero v.s. Ground Truth}
%     \label{fig:case_1}
% \end{figure*}

% \begin{figure*}[htbp]
%     \centering
%         \includegraphics[width=1\textwidth]{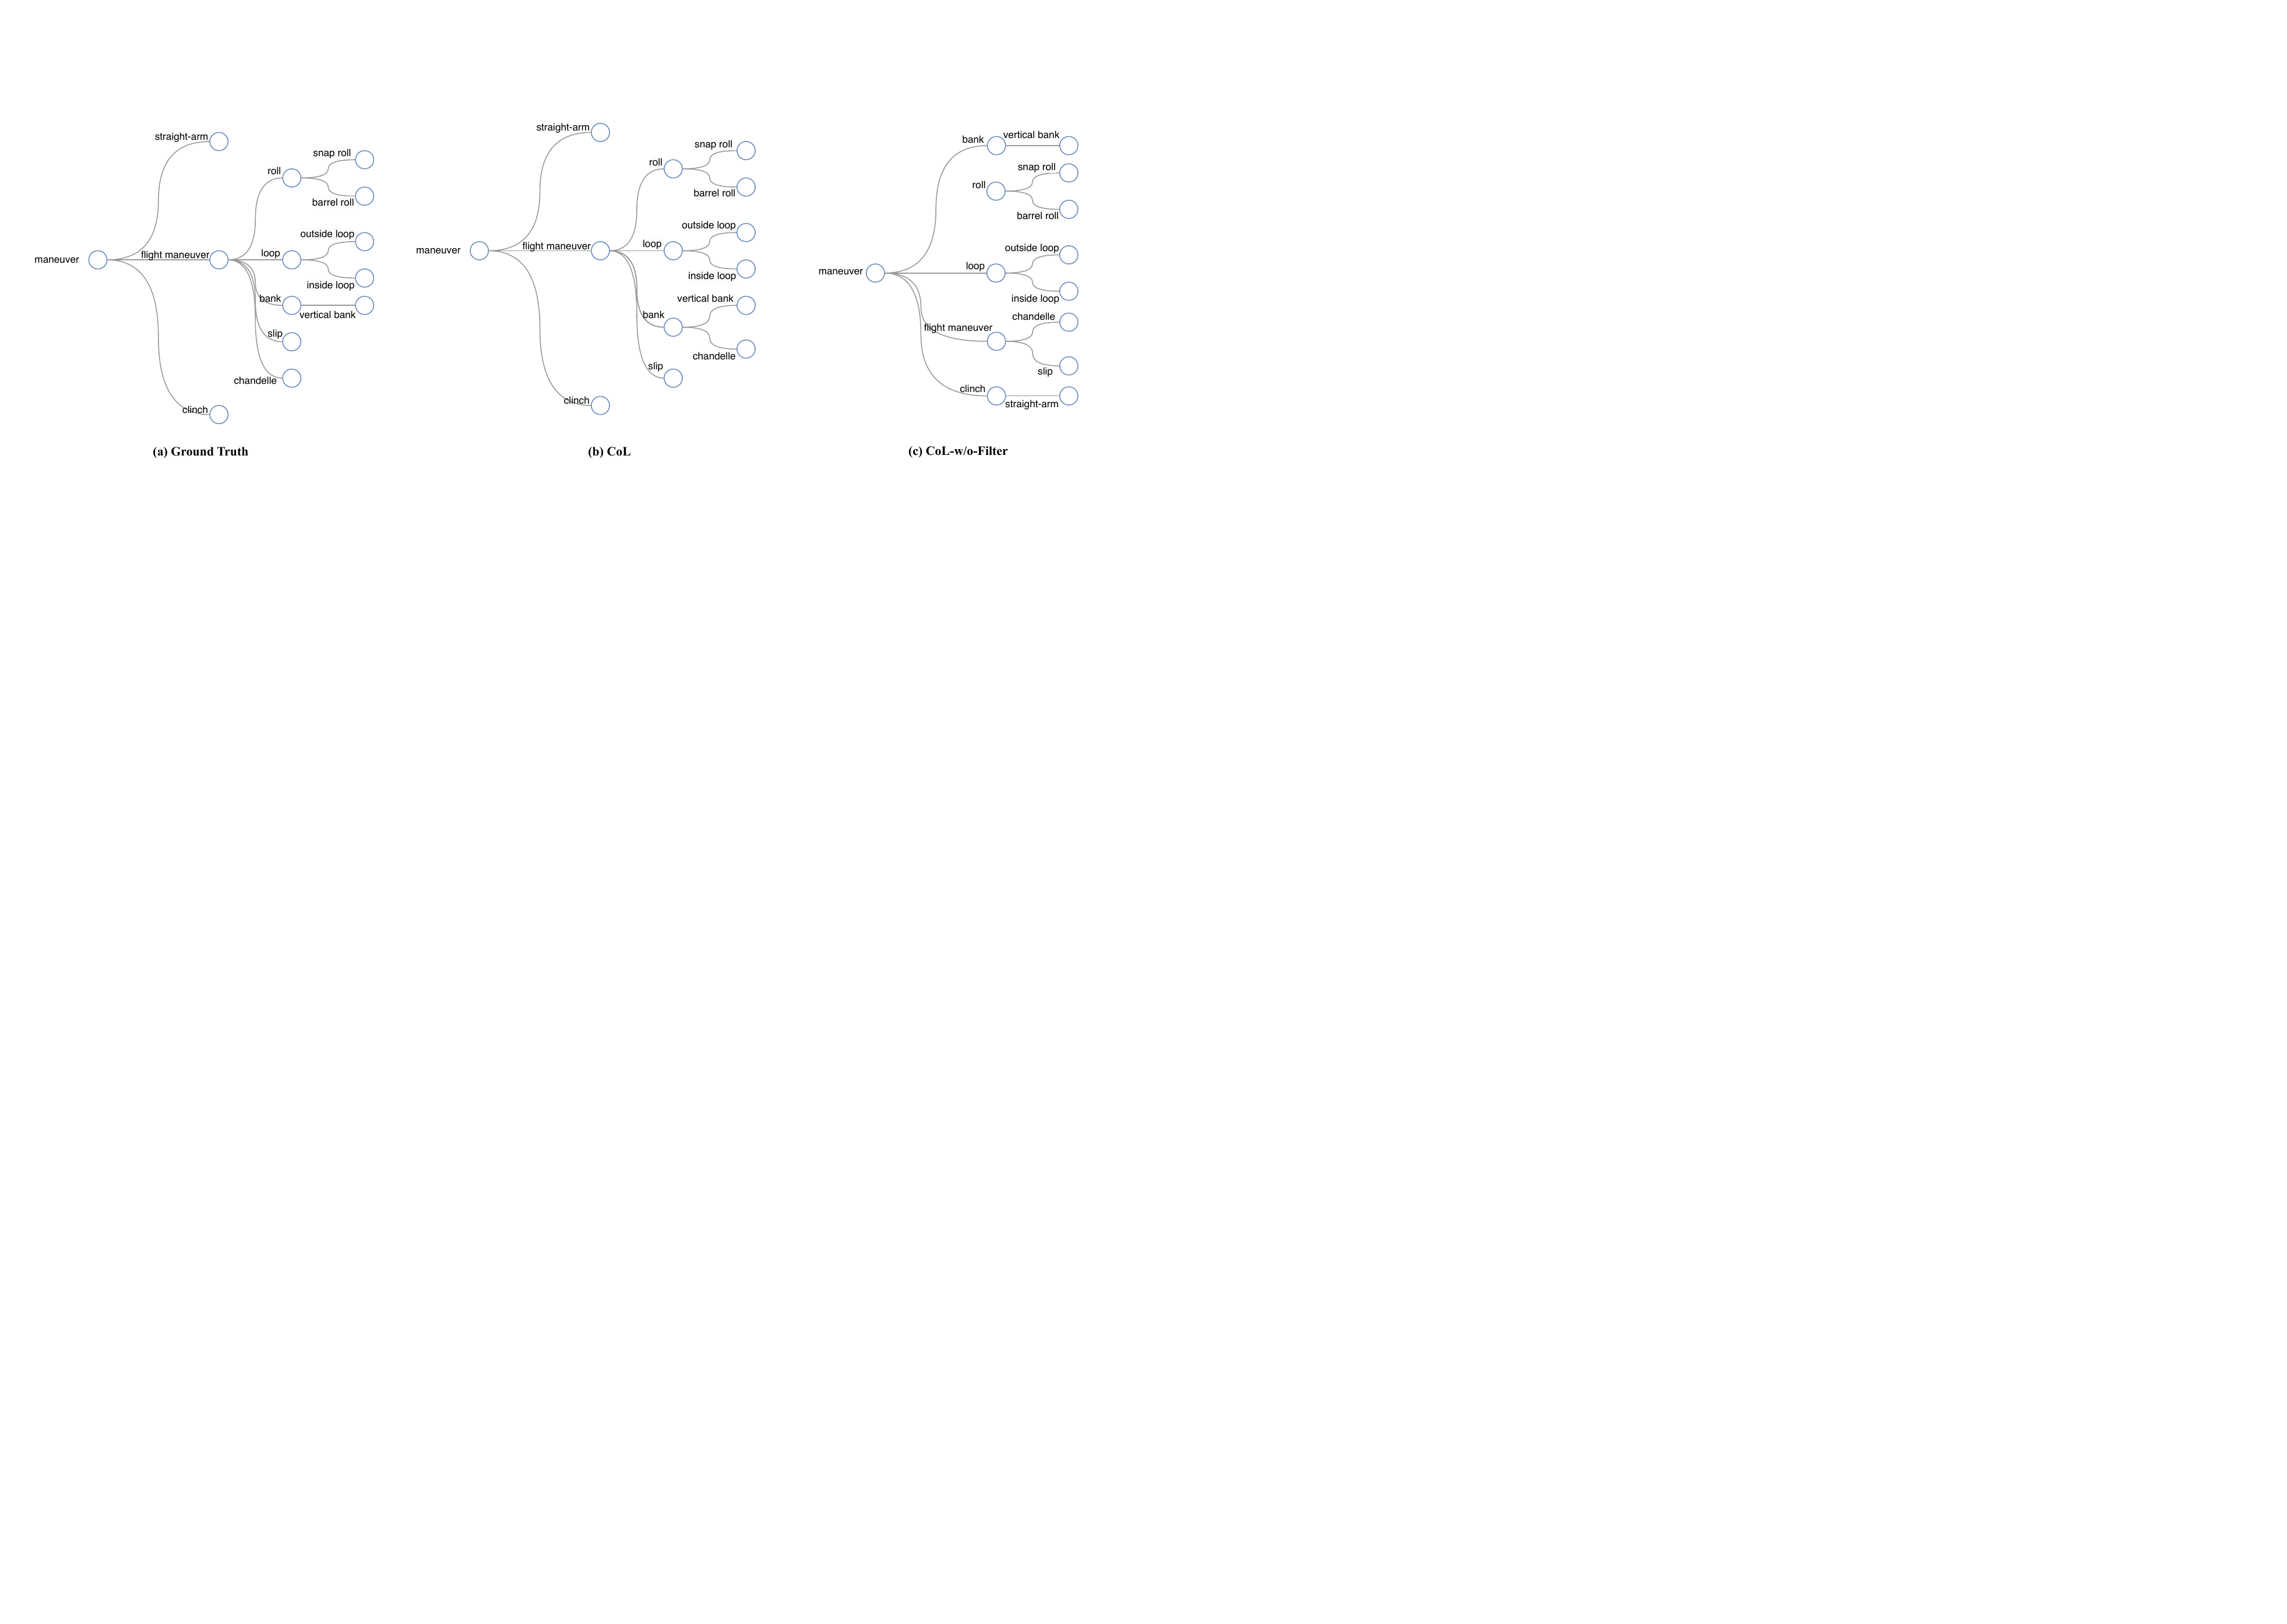}
%     \caption{CoL v.s. CoL-w/o-Filter}
%     \label{fig:case_2}
% \end{figure*}

\begin{figure*}[htbp]
    \centering
        \includegraphics[width=1\textwidth]{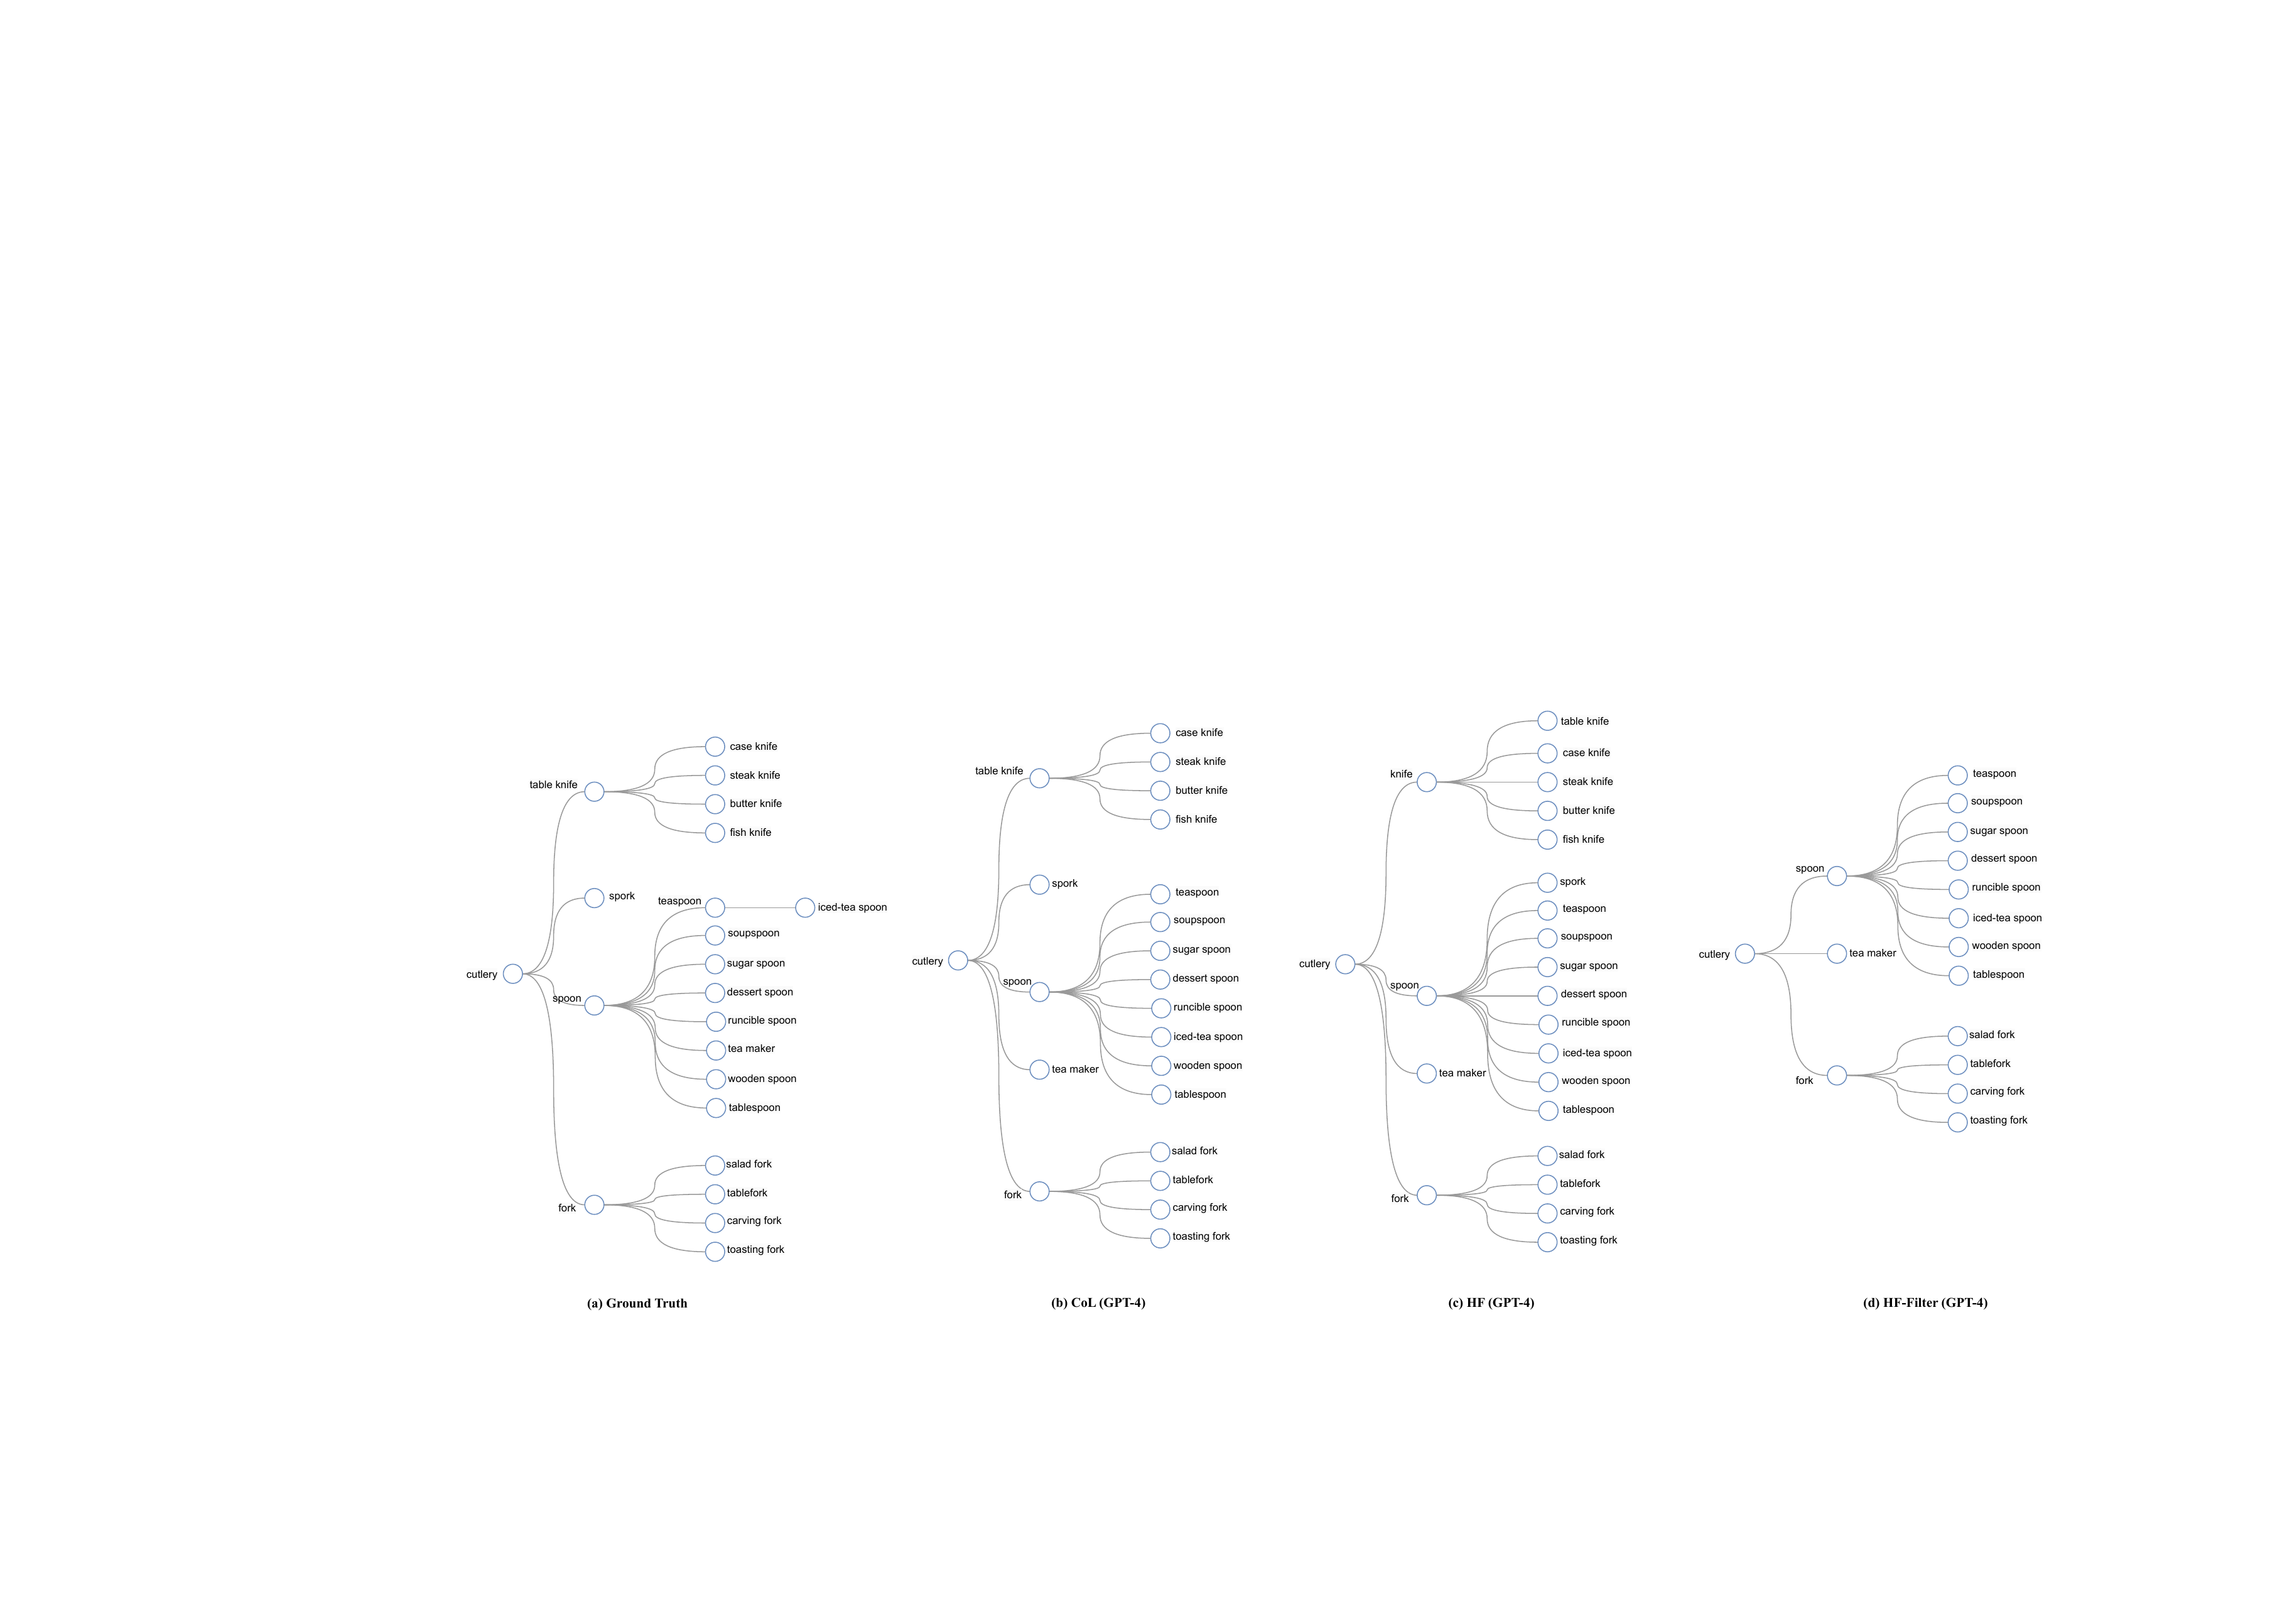}
    \caption{CoL v.s. HF (GPT-4) / HF-Filter (GPT-4)}
    \label{fig:case_3}
\end{figure*}
