# Supplementary material for: Chain-of-Layer: Iteratively Prompting Large Language Models for Taxonomy Induction from Limited Examples
Source: arXiv:2402.07386 source file (2024-07-25)
Supplement: Supplementary file 2 [file 8appendix_CoL_example.tex]

\section{Method Details}

\subsection{Algorithm of Chain-of-Layer}
The pseudo code of \textsc{Chain-of-Layer} is presented at Algorithm~\ref{alg:col}.
\begin{algorithm}
\caption{Taxonomy Induction via \textsc{Chain-of-Layer} with Ensemble-based Ranking Filter}
\begin{algorithmic}[1]
\State \textbf{Input:} $Root Entity$ $\boldsymbol{v}_0$, a root entity for the taxonomy 
\State \ \ \ \ \ \ \ \ \ \ $Entity Set$ $\mathcal{V}$, a set of entitys to be added to the taxonomy
\State \textbf{Output:} A taxonomy $\mathcal{T}$ including all entities from the set  $\mathcal{V}$

\Procedure{\textsc{Chain-of-Layer}}{$\boldsymbol{v}_0$, $\mathcal{V}$}
    \State $\mathcal{T} \gets \text{initialize $\mathcal{T}$ with} \  \boldsymbol{v}_0$
    \State $\mathcal{V}_{sel} \gets [\boldsymbol{v}_0]$
    \State $\mathcal{V} \gets \mathcal{V} \setminus \boldsymbol{v}_0$
    \State $k \gets 1$
    \While{$\mathcal{V} \text{ is not empty}$}
        \State $\mathcal{T},\mathcal{V}_{sel} \gets \textsc{CoL-K}(\mathcal{V}, \mathcal{T}, k)$
        \State $\mathcal{V}^{k} \gets \mathcal{V}^{k-1} \setminus \mathcal{V}^{k}_{sel} $
        \State $\mathcal{T},\mathcal{V} \gets \textsc{EnsembleFilter}(\mathcal{T}, \mathcal{V}, \mathcal{V}_{sel})$
        \State $k \gets k+1$
    \EndWhile
    \State \textbf{return} $\mathcal{T}$
\EndProcedure

\Procedure{\textsc{CoL-K}}{$\mathcal{V}, \mathcal{T}, k$}
    \State $\mathcal{V}_{sel} \gets \text{select all k-level entitys from} \ \mathcal{V} \ \text{for addition to}\ \mathcal{T}$
    \State $\mathcal{T} \gets \text{add } \mathcal{V}_{sel} \text{ to } \mathcal{T}$
    \State $\mathcal{V} \gets \text{remove } \mathcal{V}_{sel} \text{ from } \mathcal{V}$
    \State \textbf{return} $\mathcal{V}_{sel}, \mathcal{V}$
\EndProcedure

\Procedure{\textsc{EnsembleFilter}}{$\mathcal{T}, \mathcal{V}, \mathcal{V}_{sel}$}
    \ForAll{$\boldsymbol{v} \in \mathcal{V}_{sel}$}
        \State Compute $\textit{score}(\boldsymbol{v} | \textit{parent($\boldsymbol{v}$)}, \mathcal{M},\mathcal{V})$ using Eq. (\ref{eq:scoring})
        \State Keep $\boldsymbol{v}$ in $\mathcal{T}$ if $\textit{parent($\boldsymbol{v}$)}$ is in top ten scores
        \State \textbf{else} Remove $\boldsymbol{v}$ from $\mathcal{T}$ and add back to $\mathcal{V}$
    \EndFor
    \State \textbf{return} $\mathcal{T}, \mathcal{V}$
\EndProcedure

\end{algorithmic}
\label{alg:col}
\end{algorithm}

\subsection{Examples of the prompts and model responses}
In Table \ref{tab:example_col}, we present a taxonomy induction example with our \textsc{CoL} framework. In Table \ref{tab:example_demo}, we present one of the few-shot demonstrations that we construct and use in our experiments. In Table \ref{tab:example_large}, we present a part of the model response using \textsc{CoL} to induct the whole SemEval-Sci taxonomy, showing why LLMs can't handle large-scale taxonomies.
\label{app:process_exp}

\begin{table*}[ht]
\centering
\small
\begin{tabularx}{\textwidth}{X}
\toprule
\textbf{\makecell{Content}}\\
\midrule
\textbf{system:} You are an expert in constructing a taxonomy from a list of concepts. \\
\textbf{Demonstration:}$\mathcal{D} = [\boldsymbol{d}_1, \cdots, \boldsymbol{d}_n]$ \\
\textbf{user:} Build a taxonomy whose root concept is maneuver with the given list of entities. The format of the generated taxonomy is: 1. Parent Concept 1.1 Child Concept. Do not change any entity names when building the taxonomy. Do not add any comments. There should be one and only one root node of the taxonomy. All entities in the entity list must appear in the taxonomy and don't add any entities that are not in the entity list. \\
Entity list: ['outside loop', 'roll', 'vertical bank', 'bank', 'barrel roll', 'flight maneuver', 'straight-arm', 'clinch', 'chandelle', 'inside loop', 'loop', 'slip', 'snap roll', 'maneuver'] \\
Let's do it step by step. \\
\textbf{assistant:} First, the entity in the first level of the taxonomy is maneuver. \\
The current taxonomy is: \\
1. maneuver \\
\textbf{user:} Check: Is the remaining entity list empty? \\
\textbf{assistant:} Answer: No. \\
\addlinespace
\textbf{user:} Then, let's find all the 2-level entities from the remaining entity list. \\
\textbf{assistant:} The current taxonomy is: \\
1. maneuver \\
1.1 straight-arm \\
1.2 flight maneuver \\
1.3 clinch \\
\textbf{user:} Check: Is the remaining entity list empty? \\
\textbf{assistant:} Answer: No. \\
\addlinespace
\textbf{user:} Then, let's find all the 3-level entities from the remaining entity list. \\
\textbf{assistant:} The current taxonomy is: \\
1. maneuver \\
1.1 straight-arm \\
1.2 flight maneuver \\
1.2.1 loop \\
1.2.2 slip \\
1.2.3 roll \\
1.2.4 bank \\
1.3 clinch \\
\textbf{user:} Check: Is the remaining entity list empty? \\
\textbf{assistant:} Answer: No. \\
\addlinespace
\textbf{user:} Then, let's find all the 4-level entities from the remaining entity list. \\
\textbf{assistant:} The current taxonomy is: \\
1. maneuver \\
1.1 straight-arm \\
1.2 flight maneuver \\
1.2.1 loop \\
1.2.1.1 inside loop \\
1.2.1.2 outside loop \\
1.2.2 slip \\
1.2.3 bank \\
1.2.3.1 chandelle \\
1.2.3.2 vertical bank \\
1.2.4 roll \\
1.2.4.1 barrel roll \\
1.2.4.2 snap roll \\
1.3 clinch \\
\textbf{user:} Check: Is the remaining entity list empty? \\
\textbf{assistant:} Answer: Yes. \\
The taxonomy is complete. \\
\addlinespace
\bottomrule
\end{tabularx}
\caption{Taxonomy Induction Example with \textsc{CoL}}
\label{tab:example_col}
\end{table*}

\begin{table*}[ht]
\centering
\small
\begin{tabularx}{\textwidth}{X}
\toprule
\textbf{\makecell{Demonstration Content}}\\
\midrule
\textbf{user:} Build a taxonomy whose root concept is neuropteron with the given list of entities. The format of the generated taxonomy is: 1. Parent Concept 1.1 Child Concept. Do not change any entity names when building the taxonomy. Do not add any comments. There should be one and only one root node of the taxonomy. All entities in the entity list must appear in the taxonomy and don't add any entities that are not in the entity list. \\
Entity list: ['ant lion', 'neuropteron', 'snakefly', 'fish fly', 'brown lacewing', 'green lacewing', 'goldeneye', 'alderfly', 'lacewing', 'spongefly', 'mantispid', 'dobson'] \\
Let's do it step by step. \\
\textbf{assistant:} First, the entity in the first level of the taxonomy is neuropteron. \\
The current taxonomy is: \\
1. neuropteron \\
\textbf{user:} Check: Is the remaining entity list empty? \\
\textbf{assistant:} Answer: No. \\
\addlinespace
\textbf{user:} Then, let's find all the 2-level entities from the remaining entity list. \\
\textbf{assistant:} The current taxonomy is: \\
1. neuropteron \\
1.1 snakefly \\
1.2 spongefly \\
1.3 lacewing \\
1.4 ant lion \\
1.5 dobson \\
1.6 alderfly \\
1.7 fish fly \\
1.8 mantispid \\
\textbf{user:} Check: Is the remaining entity list empty? \\
\textbf{assistant:} Answer: No. \\
\addlinespace
\textbf{user:} Then, let's find all the 3-level entities from the remaining entity list. \\
\textbf{assistant:} The current taxonomy is: \\
1. neuropteron \\
1.1 snakefly \\
1.2 spongefly \\
1.3 lacewing \\
1.3.1 brown lacewing \\
1.3.2 green lacewing \\
1.4 ant lion \\
1.5 dobson \\
1.6 alderfly \\
1.7 fish fly \\
1.8 mantispid \\
\textbf{user:} Check: Is the remaining entity list empty? \\
\textbf{assistant:} Answer: No. \\
\addlinespace
\textbf{user:} Then, let's find all the 4-level entities from the remaining entity list. \\
\textbf{assistant:} The current taxonomy is: \\
1. neuropteron \\
1.1 snakefly \\
1.2 spongefly \\
1.3 lacewing \\
1.3.1 brown lacewing \\
1.3.2 green lacewing \\
1.3.2.1 goldeneye \\
1.4 ant lion \\
1.5 dobson \\
1.6 alderfly \\
1.7 fish fly \\
1.8 mantispid \\
\textbf{user:} Check: Is the remaining entity list empty? \\
\textbf{assistant:} Answer: Yes. \\
The taxonomy is complete. \\
\bottomrule
\end{tabularx}
\caption{\textsc{CoL} Demonstration Example}
\label{tab:example_demo}
\end{table*}

\begin{table*}[ht]
\centering
\small
\begin{tabularx}{\textwidth}{X}
\toprule
\textbf{\makecell{Content}}\\
\midrule
\textbf{[Previous Iterations]}\\
\addlinespace
\textbf{user:} Then, let's find all the 4-level entities from the remaining entity list. \\
\textbf{assistant:} The current taxonomy is: \\
1. science\\
1.1 Natural Sciences\\
1.1.1 Physics\\
1.1.1.1 Quantum Physics\\
1.1.1.2 Solid State Physics\\
1.1.1.3 Nuclear Physics\\
1.1.1.4 Thermodynamics\\
1.1.1.5 Mechanics\\
1.1.1.6 Optics\\
1.1.2 Chemistry\\
1.1.2.1 Organic Chemistry\\
1.1.2.2 Inorganic Chemistry\\
1.1.2.3 Biochemistry\\
1.1.2.4 Physical Chemistry\\
1.1.3 Earth Science\\
1.1.3.1 Geophysics\\
1.1.3.2 Seismology\\
1.1.3.3 Volcanology\\
1.1.3.4 Paleontology\\
1.1.4 Space Science\\
1.1.4.1 Astronomy\\
1.1.4.2 Astrophysics\\
1.1.4.3 Cosmology\\
1.1.5 Biology\\
1.1.5.1 Zoology\\
1.1.5.1.1 Entomology\\
1.1.5.1.2 Ichthyology\\
1.1.5.1.3 Ornithology\\
1.1.5.2 Botany\\
1.1.5.3 Microbiology\\
1.1.5.3.1 Bacteriology\\
1.1.5.4 Genetics\\
1.2 Formal Sciences\\
1.2.1 Mathematics\\
1.2.1.1 Algebra\\
1.2.1.2 Calculus\\
1.2.1.3 Geometry\\
1.2.2 Computer Science\\
1.2.2.1 Computational Linguistics\\
1.2.2.2 Artificial Intelligence\\
1.2.3 Logic\\
\textbf{[...]}\\
\addlinespace
\textbf{user:} Check: Is the remaining entity list empty?\\
\textbf{assistant:} Answer: No.
The process continues until all entities in your list have been placed into the taxonomy under the appropriate sub-categories, continuing to break them down into more specific fields of study and disciplines. Given the vast number of entities provided and the complexity of categorizing them, a complete taxonomy is beyond the scope of this interaction. However, the demonstrated approach should give a clear idea of how to proceed.\\
\bottomrule
\end{tabularx}
\caption{An example of LLMs can not handle large-scale taxonomy}
\label{tab:example_large}
\end{table*}
